# Supplementary material for: Waffling around for Performance: Visual Classification with Random Words and Broad Concepts
Source: arXiv:2306.07282 source file (2023-08-17)
Supplement: Supplementary file 1 [file additional_benchmarks_sup.tex]

\begin{table}[t]
\centering\resizebox{0.48\textwidth}{!}{
\begin{tabular}{l|lll|l}
\toprule
\textbf{ViT-B/32} & Flowers102 & FGVCAircraft & Stanford Cars & \textbf{Avg} \\
\hline
CLIP & 62.89 & 24.99 & 58.54 & 48.81\\
DCLIP \cite{dclip} & 64.01 & 26.94 & 57.08 & 49.34\\

\hline
\texttt{Waffle}CLIP & 66.27 \small$\pm0.26$ & 25.66 \small$\pm0.19$ & 58.91 \small$\pm0.17$ & 50.28 \small$\pm0.21$\\
+ Concepts & \textbf{67.19} \small$\pm0.19$ & 28.44 \small$\pm0.22$ & \textbf{59.70} \small$\pm0.12$ & \blue{\textbf{51.78}} \small$\pm0.18$\\
+ GPT dsc. + Conc. & 66.71 \small$\pm0.39$ & \textbf{28.96} \small$\pm0.37$ & 59.33 \small$\pm0.14$ & 51.67 \small$\pm0.32$\\
\bottomrule
\end{tabular}
}
\centering\resizebox{0.48\textwidth}{!}{
\begin{tabular}{l|lll|l}
\toprule
\textbf{ViT-L/14} & Flowers102 & FGVCAircraft & Stanford Cars & \textbf{Avg} \\
\hline
CLIP & 74.73 & 44.88 & 76.42 & 65.34\\
DCLIP \cite{dclip} & 78.16 & \textbf{51.04} & 75.13 & 68.11\\
\hline
\texttt{Waffle}CLIP & 76.17 \small$\pm0.27$ & 48.72 \small$\pm0.40$ & \textbf{76.71} \small$\pm0.12$ & 67.20 \small$\pm0.29$\\
+ Concepts & 78.12 \small$\pm0.18$ & 49.45 \small$\pm0.26$ & 76.41 \small$\pm0.08$ & 67.99 \small$\pm0.19$\\
+ GPT dsc. + Conc. & \textbf{78.57} \small$\pm0.22$ & 50.79 \small$\pm0.47$ & 76.23 \small$\pm0.14$ & \blue{\textbf{68.53}} \small$\pm0.31$\\
\bottomrule
\end{tabular}
}
\centering\resizebox{0.48\textwidth}{!}{
\begin{tabular}{l|lll|l}
\toprule
\textbf{ResNet50} & Flowers102 & FGVCAircraft & Stanford Cars & \textbf{Avg} \\
\hline
CLIP & 61.36 & 21.15 & 54.05 & 45.52\\
DCLIP \cite{dclip} & 64.86 & 24.48 & 52.59 & 47.31\\
\hline
\texttt{Waffle}CLIP & 65.25 \small$\pm0.34$ & 23.66 \small$\pm0.04$ & 53.77 \small$\pm0.23$ & 47.56 \small$\pm0.24$\\
+ Concepts & 66.58 \small$\pm0.20$ & 24.25 \small$\pm0.09$ & \textbf{54.11} \small$\pm0.23$ & 48.31 \small$\pm0.18$\\
+ GPT dsc. + Conc. & \textbf{67.11} \small$\pm0.24$ & 24.80 \small$\pm0.32$ & 53.64 \small$\pm0.12$ & \blue{\textbf{48.52}} \small$\pm0.24$\\
\bottomrule
\end{tabular}
}
\caption{We find consistent performance improvements with \ourmodel, and when utilizing additional high-level concept guidance in three additional benchmarks. Some benchmarks may not benefit from additional descriptors (see \textit{Stanford Cars}), but high-level concepts or \texttt{Waffle}CLIP still prove useful.}
\label{sup:tab:additional_benchmarks}
\end{table}
