# Supplementary material for: Waffling around for Performance: Visual Classification with Random Words and Broad Concepts
Source: arXiv:2306.07282 source file (2023-08-17)
Supplement: Supplementary file 2 [file supp_motivation.tex]

\begin{table*}[t]
\centering\resizebox{0.98\textwidth}{!}{
\begin{tabular}{l|llllllll|l}
\toprule
\textbf{ViT-B/32} & ImageNetV2 & ImageNet & CUB200 & EuroSAT & Places365 & Food101 & Oxford Pets & DTD & \textbf{Avg}\\
\hline
CLIP~\cite{clip} &  54.71 & 62.01 & 51.28 & 40.78 & 39.12 & 82.59 & 85.06 & 43.18 & 57.34 \\
DCLIP~\cite{dclip} &  \textbf{55.82} & \textbf{63.12} & 52.47 & \textbf{43.29} & 40.47 & 82.79 & 86.54 & \textbf{43.99} & \blue{\textbf{58.56}}\\
\hline
DCLIP (same, 1x)  & 55.47 \small$\pm0.24$ & 62.89 \small$\pm0.19$ & 52.64 \small$\pm0.28$ & 39.74 \small$\pm2.69$ & 40.29 \small$\pm0.47$ & 83.82 \small$\pm0.48$ & 87.04 \small$\pm0.27$ & 43.35 \small$\pm0.41$ & 58.16 \small$\pm1.01$\\
DCLIP (same, 2x) & 55.75 \small$\pm0.21$ & 63.10 \small$\pm0.19$ & \textbf{52.72} \small$\pm0.23$ & 39.73 \small$\pm1.66$ & \textbf{40.61} \small$\pm0.22$ & \textbf{84.01} \small$\pm0.23$ & \textbf{87.10} \small$\pm0.14$ & 43.29 \small$\pm0.22$ & 58.29 \small$\pm0.62$\\
\bottomrule
\end{tabular}
}
\centering\resizebox{0.98\textwidth}{!}{
\begin{tabular}{l|llllllll|l}
\toprule
\textbf{ResNet50} & ImageNetV2 & ImageNet & CUB200 & EuroSAT & Places365 & Food101 & Oxford Pets & DTD & \textbf{Avg}\\
\hline
CLIP~\cite{clip} &  51.34 & 58.16 & 45.20 & 28.09 & 36.63 & 78.37 & 83.76 & 38.51 & 52.51\\
DCLIP~\cite{dclip} &  52.70 & 59.66 & \textbf{47.76} & 34.27 & 38.39 & 78.59 & \textbf{85.77} & \textbf{41.01} & 54.77\\
\hline
DCLIP (same, 1x) & 52.63 \small$\pm0.28$ & 59.69 \small$\pm0.30$ & \textbf{47.76} \small$\pm0.39$ & 32.74 \small$\pm1.49$ & 38.63 \small$\pm0.22$ & 80.08 \small$\pm0.58$ & 85.36 \small$\pm0.52$ & 40.77 \small$\pm0.63$ & 54.71 \small$\pm0.67$\\
DCLIP (same, 1x) & \textbf{52.89} \small$\pm0.23$ & \textbf{59.90} \small$\pm0.26$ & 47.70 \small$\pm0.29$ & \textbf{34.37} \small$\pm1.27$ & \textbf{38.93} \small$\pm0.21$ & \textbf{80.11} \small$\pm0.30$ & 85.34 \small$\pm0.29$ & 40.91 \small$\pm0.79$ & \blue{\textbf{55.02}} \small$\pm0.58$\\
\bottomrule
\end{tabular}
}
\caption{\textbf{Motivating random class descriptors.} Comparing CLIP~\cite{clip} and GPT-descriptor-extended CLIP~\cite{dclip} (DCLIP) with the same set of randomly sampled descriptors used for each class, where the set size is either the average number of descriptions per class in DCLIP (\textit{same, 1x}), or twice that (\textit{same, 2x}). 
%Note that unlike \cite{dclip}, we utilize the \texttt{"A photo of a \{c\}."} prompt in all cases for a fair comparison. 
A random set of descriptors per class can match or even outperform DCLIP 
% the class-specific GPT-3 generated descriptor extension (e.g.\ \texttt{"A photo of a [waffle], which is [a round shape]."}) 
across backbone architectures confirming that randomized prompt averaging leads to higher performance.}
\label{tab:motivation}
\end{table*}
